# Supplementary material for: HippoSpark: An On-Demand Experience System for LLM Reasoning
Source: arXiv:2606.29929 source file (2026-06-29)
Supplement: Supplementary file 1 [file prompt.tex]

\section{Prompt Templates}
\label{app:prompts}
\dl{
Provide the full prompt templates referenced earlier. Organize them by function, such as transition assessment, bottleneck analysis, experience construction, retrieval-augmented next-move generation, and verification. This section should contain the exact prompts used in experiments.
}

This section presents the \emph{universal prompt templates} used in the experience-construction stage.

Instead of enumerating benchmark-specific prompts separately, we abstract a shared template for each functional role and then describe how it is specialized for MATH, GPQA, and BigCodeBench.

\begin{tcolorbox}[
    breakable,
    colback=white!98!black,
    colframe=black!70!white,
    boxsep=4pt,
    top=2pt,
    title={\textbf{\large Function I: Transition Assessment / Bottleneck Analysis}},
    coltitle=black,
    colbacktitle=gray!20,
    bottom=2pt
]

\textbf{Trajectory Pivot and Bottleneck Analysis Prompt Template}
\begin{lstlisting}[style=plainoutput]
You are an expert in {domain} reasoning analysis.

[Context]
The provided trajectory led to a {outcome} result.
Task / Problem: {problem}
Auxiliary Context: {auxiliary_context}

[Trajectory]
{trajectory}

[Task]
1. Identify the most essential domain anchors used at the key turning points.
   - Use canonical naming whenever possible.
   - Avoid trivial or generic tags.

2. Conduct a step-by-step analysis of the trajectory.
   You MUST explicitly mark key turning points using the tag [PIVOT].

3. For each [PIVOT], explain:
   (a) the bottleneck / barrier / hidden constraint,
   (b) the key anchor that resolves it,
   (c) the reasoning function or decision role of this pivot.

[Output Format]
<ANCHOR_BLOCK>
[Domain Anchor 1]
[Domain Anchor 2]
...
</ANCHOR_BLOCK>

<analysis>
[PIVOT] At step X, the solver faced [Barrier]. Applying [Anchor] enabled [Resolution]. 
This pivot mainly served [Decision Role].
</analysis>
\end{lstlisting}

\end{tcolorbox}

Although all three benchmarks share the same high-level structure of identifying critical pivots and diagnosing bottlenecks from trajectories, their concrete analytical focus differs substantially.

For MATH, the template is specialized around \emph{theoretical anchors}, requiring the model to extract theorems, lemmas, structural observations, or algorithmic principles that resolve the key obstacles in the solution process. The analysis emphasizes how each pivot corresponds to a mathematically meaningful barrier and how that barrier is overcome through a formal conceptual tool.

For GPQA, the same pivot-analysis backbone is preserved, but the anchors are redefined as scientific principles, mechanisms, or discriminative criteria. In addition, the template explicitly strengthens the notion of \emph{decision role}, so that each pivot is not only explained in terms of how it advances reasoning, but also in terms of whether it identifies the governing principle, eliminates distractors, or corrects a misconception.

For BigCodeBench, the template is further grounded in execution feedback, test behavior, and concrete implementation traces. As a result, bottleneck analysis is no longer restricted to abstract reasoning transitions, but is instead tied to implementation decisions, hidden constraints, failure symptoms, and root causes of incorrect code behavior. A Python technique or API usage is promoted to an anchor only when it is genuinely critical to the success or failure of the attempt.

\begin{tcolorbox}[
    breakable,
    colback=white!98!black,
    colframe=black!70!white,
    boxsep=4pt,
    top=2pt,
    title={\textbf{\large Function II: Knowledge Consolidation}},
    coltitle=black,
    colbacktitle=gray!20,
    bottom=2pt
]

\textbf{Unknowledge Consolidation Prompt Template}
\begin{lstlisting}[style=plainoutput]
You are a {domain} knowledge engineer.

[Input]
Raw list of anchors extracted from reasoning pivots:
{anchors}

[Task Process]
Step 1: Normalization and Clustering
- Merge synonyms, variants, and conceptually identical items.
- Assign one canonical name to each cluster.

Step 2: Filtering
- Remove generic, noisy, or uninformative items.
- Keep only reusable domain principles, methods, or patterns.

Step 3: Structured Card Generation
- Convert each valid cluster into a structured reusable card.

[Output Format]
### Step 1: Clustering Map
[Canonical Name] <= [raw mentions]

### Step 2: Filtering Log
- KEPT: ...
- DISCARDED: ...

### Step 3: Structured Cards
<knowledge_card>
Name: ...
Field / Type: ...
Definition / Correct_Pattern: ...
Core_Criterion / Formula / Usage: ...
Key_Insight / Common_Confusion / Pitfall: ...
</knowledge_card>
\end{lstlisting}

\end{tcolorbox}

The three benchmarks follow the same overall pipeline of normalization, filtering, and card construction, but the schema of the resulting knowledge cards is systematically adapted to the nature of the task.

For MATH, the cards are designed to support formal reasoning reuse, and therefore emphasize \emph{Definition}, \emph{Formula}, and \emph{Key Insight}, preserving the exact meaning of a theorem or structural method together with its mathematical expression.

For GPQA, the cards are intended to support mechanism identification and option discrimination rather than symbolic derivation. Accordingly, they place greater emphasis on \emph{Core Criterion}, \emph{Typical Use}, and \emph{Common Confusion}, so that the stored knowledge directly answers when a principle applies, how it distinguishes competing explanations, and what misconceptions it helps avoid.

For BigCodeBench, the knowledge objects shift from abstract principles to executable methods.
The cards are therefore specialized into method cards that foreground \emph{when to use}, \emph{correct pattern}, \emph{pitfall and symptom}, and minimal reusable code snippets.
This design allows later experience units to cleanly separate strategy-level decision making from implementation-level execution details.

\begin{tcolorbox}[
    breakable,
    colback=white!98!black,
    colframe=black!70!white,
    boxsep=4pt,
    top=2pt,
    title={\textbf{\large Function III: Experience Construction}},
    coltitle=black,
    colbacktitle=gray!20,
    bottom=2pt
]

\textbf{Experience Construction Prompt Template}
\begin{lstlisting}[style=plainoutput]
You are a {domain} strategy architect / experience engineer.

[Input]
Expert Analysis: {analysis}
Knowledge Cards / Method Cards: {knowledge_points}

[Goal]
Decompose the input into multiple reusable experience units.
Each unit should capture:
(1) what kind of situation is being recognized,
(2) what the true strategic goal is,
(3) what execution kernel or action kernel should be applied,
(4) how the cited knowledge cards are adapted.

[Alignment Rule]
The experience will be retrieved using:
"Situation: [Context] + Quest: [Target]"

[Output Format]
<experience>
  <id>[Unique ID]</id>
  <type>[Strategy Model | Constraint Trap | Misleading Pattern | ...]</type>

  <situation_signature>[Abstract problem situation]</situation_signature>
  <strategic_goal>[What must be solved, preserved, distinguished, or avoided]</strategic_goal>

  <execution_kernel_or_action_kernel>
    [Step 1 ...]
    [Step 2 ...]
    [Step 3 ...]
  </execution_kernel_or_action_kernel>

  <cited_methods>
    [Exact card name 1: adaptation logic]
    [Exact card name 2: adaptation logic]
  </cited_methods>
</experience>
\end{lstlisting}

\end{tcolorbox}

At the final experience-construction stage, all three benchmarks share the same objective: to compress trajectory analysis and structured knowledge into reusable experience units that can be retrieved through a unified Situation and Quest interface. However, the semantic emphasis of the resulting experience units differs across domains.

For MATH, each experience unit is specialized into a strategy card for abstract mathematical situations, focusing on when a particular mathematical tool should be invoked under a given structural condition and how that tool supports problem reduction through formal derivation.

For GPQA, the experience units are shaped as scientific discrimination templates. Their primary purpose is not to reproduce a full solution, but to identify the governing principle, extract the decisive criterion, and use that criterion to eliminate superficially plausible but mechanistically incorrect distractors.

For BigCodeBench, the experience units are further organized into a two-layer structure. The upper layer determines which implementation strategy should be selected based on task signals, input-output constraints, and test-level symptoms, while the lower layer delegates concrete coding patterns and API usage to the associated method cards.

This section next presents the \emph{universal prompt templates} used in the experience-utilization stage. Compared with experience construction, experience utilization involves online planning, retrieval triggering, memory-grounded next-step generation, and runtime verification.

Instead of enumerating benchmark-specific prompts separately, we abstract a shared template for each functional role and then describe how it is specialized for MATH, GPQA, and BigCodeBench.

\begin{tcolorbox}[
    breakable,
    colback=white!98!black,
    colframe=black!70!white,
    boxsep=4pt,
    top=2pt,
    title={\textbf{\large Function IV: Problem Profiling / Constraint Extraction}},
    coltitle=black,
    colbacktitle=gray!20,
    bottom=2pt
]

\textbf{Problem Profiling / Constraint Extraction Prompt Template}
\begin{lstlisting}[style=plainoutput]
You are a task profiler for {domain} problem solving.

[Input]
Problem:
{problem}

Optional Context:
{auxiliary_context}

[Task]
Before any retrieval or execution, identify the reasoning frame and the hard constraints
that should govern subsequent decision making.

Focus on:
1. Task type / reasoning style / operator.
2. Structural constraints or interface requirements.
3. Likely traps, ambiguity sources, or discriminative dimensions.
4. The expected answer form or output format.

[Output Format]
<profile>
Task_Type: ...
Reasoning_Frame: ...
Key_Constraints: ...
Likely_Traps: ...
Answer_or_Output_Form: ...
</profile>
\end{lstlisting}

\end{tcolorbox}

For MATH, this function is largely implicit rather than instantiated as a separate prompt.
The mathematical solving process is framed directly through the planner's state-transition representation, where the current verified state, the next subgoal, and the gap type together serve as the operative problem profile.

For GPQA, this function is explicitly specialized into a structured problem profiler.
Rather than extracting formal interface constraints, it characterizes the scientific reasoning frame: domain, question style, operator, option-role patterns, likely governing principles, discriminative axes, and common traps.
This design reflects the fact that GPQA success depends heavily on recognizing how answer options should be distinguished before any detailed reasoning is attempted.

For BigCodeBench, the profiling stage is specialized into requirement and interface extraction.
Instead of modeling abstract reasoning frames, it focuses on the exact entry point, function signature, argument structure, return format, and task-level constraints such as edge cases or complexity hints.
This adaptation is necessary because downstream code generation must be tightly aligned with executable interfaces rather than only conceptual task structure.

\begin{tcolorbox}[
    breakable,
    colback=white!98!black,
    colframe=black!70!white,
    boxsep=4pt,
    top=2pt,
    title={\textbf{\large Function V: Retrieval-Augmented Next-Move Generation}},
    coltitle=black,
    colbacktitle=gray!20,
    bottom=2pt
]

\textbf{Retrieval-Augmented Next-Move Generation Prompt Template}
\begin{lstlisting}[style=plainoutput]
You are the Cortex / Planner for {domain} problem solving.

[Current Input]
Problem: {problem}
Current State / Latest Tool Output: {state}

[Decision Protocol]
At each turn:
1. Analyze the current state using observation only.
2. Identify the immediate subgoal or target next state.
3. Determine the dominant gap:
   - strategic gap,
   - computational / executable gap,
   - local mechanical reasoning gap,
   - or completion.
4. Choose exactly one action:
   - <memory> / <memory_query> when retrieval is needed,
   - <calc> / <move> / <plan> when the next step is executable,
   - <answer> only when the final output is ready.

[Output Format]
Reasoning:
1. Current frame
2. Immediate uncertainty / gap
3. Why the chosen action is the best next step

Action:
<memory>...</memory>
OR
<memory_query>...</memory_query>
OR
<calc>...</calc>
OR
<move>...</move>
OR
<plan>...</plan>
OR
<answer>...</answer>
\end{lstlisting}

\end{tcolorbox}

Although all three benchmarks share the same high-level planner structure of observing the current state, identifying the next subgoal, and deciding whether retrieval is needed, the action space is specialized to the demands of each domain.

For MATH, the planner is cast explicitly as a state-transition controller.
The key distinction is between a \emph{strategy gap} and a \emph{calculation gap}: strategic gaps trigger memory retrieval, whereas computational gaps trigger a calculator request.
The planner is also instructed to describe state transitions in terms of verified current state, target next state, and the bridge needed between them, which makes the retrieval decision tightly coupled to mathematical problem decomposition.

For GPQA, the planner is specialized for scientific multiple-choice reasoning.
In addition to memory retrieval and optional calculation, it introduces a dedicated \texttt{<move>} action for local executable reasoning steps such as comparison, elimination, or one-step derivation.
This reflects the fact that GPQA often requires not a full strategy overhaul, but a single discriminative check that advances the answer-selection process.
The planner therefore emphasizes identifying the decisive uncertainty and choosing whether it is best resolved by experience retrieval, lightweight reasoning, or computation.

For BigCodeBench, the planner is adapted to implementation-oriented problem solving.
Instead of directly producing code, it chooses between \texttt{<memory\_query>} and \texttt{<plan>}.
The former is used when the model is uncertain about APIs, hidden edge cases, or specific failure patterns, while the latter serves as a structured implementation blueprint for the downstream coding expert.
This makes the planner less about deriving answers directly and more about orchestrating a robust transition from abstract task understanding to executable program synthesis.

\begin{tcolorbox}[
    breakable,
    colback=white!98!black,
    colframe=black!70!white,
    boxsep=4pt,
    top=2pt,
    title={\textbf{\large Function VI: Memory Query Formulation}},
    coltitle=black,
    colbacktitle=gray!20,
    bottom=2pt
]

\textbf{Memory Query Formulation Prompt Template}
\begin{lstlisting}[style=plainoutput]
You are the memory query generator for {domain} reasoning.

[Input]
Current state / blockage:
{state}

[Task]
Convert the current blockage into retrieval-friendly query language for an
experience database indexed by abstract situation and goal.

Requirements:
1. Describe the structural situation, not superficial wording.
2. State the missing bridge, discriminator, or objective.
3. Avoid directly proposing a complete solution or final answer.
4. Generate concise, retrieval-oriented queries.

[Output Format]
<analysis>
[Why this is the right abstraction of the blockage]
</analysis>

<queries>
<query>Situation: [Context] | Goal / Gap / Quest: [Objective]</query>
</queries>
\end{lstlisting}

\end{tcolorbox}

The three benchmarks all require retrieval queries to be expressed at a level that matches reusable experience units, but the abstraction granularity differs by domain.

For MATH, query formulation is specialized around \emph{strategic bridges}.
The query does not merely restate the problem, but explicitly isolates the mathematical structure, the missing link, and the type of theorem, transformation, or simplification needed.
In the actual implementation, MATH further refines this process by rewriting raw retrieval requests into generalized two-line \emph{Situation} and \emph{Quest} forms so that the query aligns with the experience library's abstract indexing scheme.

For GPQA, memory query generation is made deliberately lightweight.
Rather than invoking a separate elaborate query generator, the planner is encouraged to issue the raw scientific need directly in \texttt{Situation + Quest} form.
This design choice reflects the importance of preserving the exact discriminative blockage, such as an unresolved mechanism contrast or an unclear governing principle, without over-normalizing it into generic retrieval language.

For BigCodeBench, query formulation is specialized around implementation context and failure signals.
The query generator is explicitly discouraged from naming a concrete algorithm and instead asked to describe the abstract coding situation: input structure, required behavior, hidden constraints, or exact error patterns such as tracebacks and malformed-data cases.
This helps retrieval focus on reusable programming experiences rather than surface-level solution keywords.

\begin{tcolorbox}[
    breakable,
    colback=white!98!black,
    colframe=black!70!white,
    boxsep=4pt,
    top=2pt,
    title={\textbf{\large Function VII: Memory-Grounded Next-Step Synthesis}},
    coltitle=black,
    colbacktitle=gray!20,
    bottom=2pt
]

\textbf{Memory-Grounded Next-Step Synthesis Prompt Template}
\begin{lstlisting}[style=plainoutput]
You are the memory synthesizer / expert consultant for {domain} reasoning.

[Input]
Current status / target goal:
{status}

Retrieved experiences:
{retrieved_info}

[Task]
1. Assess whether the retrieved experience is relevant and sufficient.
2. If relevant, adapt it to the current state rather than repeating it verbatim.
3. If incomplete or weakly relevant, supplement or partially replace it with
   domain knowledge while keeping the output focused on the immediate next step.
4. Do not jump to the final answer unless explicitly required by the task design.

[Output Format]
<analysis>
[Relevance judgment + what is adopted / supplemented]
</analysis>

<suggestion_or_experience>
[The concrete next-step reasoning, adapted strategy, or preserved-and-completed experience]
</suggestion_or_experience>
\end{lstlisting}

\end{tcolorbox}

All three benchmarks use retrieval not as a source of final answers, but as a source of intermediate guidance that must be adapted to the current blockage.
However, what counts as a valid adaptation differs substantially.

For MATH, memory synthesis is specialized toward preserving the original retrieved mathematical experience while supplementing missing formulas, omitted steps, or key constraints.
The emphasis is on maintaining the structure of the retrieved strategy while making it sufficiently complete and actionable for the current mathematical goal.
This reflects the dense and formula-sensitive nature of mathematical experience reuse.

For GPQA, memory synthesis is specialized into \emph{next-step reasoning generation}.
The synthesizer is explicitly forbidden from outputting a final answer option and instead must convert retrieved experience into a single scientifically meaningful next step together with its intermediate conclusion.
If the retrieved text itself suggests an answer option, that signal is treated as untrusted and must be transformed into checks, comparisons, or criterion-based reasoning.
This design ensures that memory supports discriminative reasoning without collapsing directly into answer prediction.

For BigCodeBench, memory synthesis is specialized into context-aware technical consulting.
Retrieved programming experiences must be rewritten using the exact variable names, data structures, API calls, and edge-case requirements relevant to the current coding state.
The output is not a full program, but an adapted sub-strategy that the planner can immediately convert into a concrete implementation plan.
As a result, retrieval serves as a bridge from generic programming knowledge to highly localized implementation decisions.

\begin{tcolorbox}[
    breakable,
    colback=white!98!black,
    colframe=black!70!white,
    boxsep=4pt,
    top=2pt,
    title={\textbf{\large Function VIII: Verification}},
    coltitle=black,
    colbacktitle=gray!20,
    bottom=2pt
]

\textbf{Verification Prompt Template}
\begin{lstlisting}[style=plainoutput]
You are the verifier for {domain} problem solving.

[Input]
Current state / trace:
{state_or_trace}

Proposed action / move / artifact:
{proposal}

Task:
1. Check whether the proposal is executable and aligned with the current goal.
2. Reject only for concrete, actionable issues.
3. Do not solve the whole task from scratch.
4. Return either approval or minimal corrective feedback.

[Output Format]
<analysis>
[Brief diagnostic rationale]
</analysis>

Action:
<valid>APPROVED</valid>
OR
<reject>[Concrete fix]</reject>
OR
<revise>[Targeted refinement instructions]</revise>
\end{lstlisting}

\end{tcolorbox}

Verification plays a common role across all three benchmarks—preventing invalid state transitions—but is instantiated at different granularities depending on the domain.

For MATH, verification is specialized as \emph{state-transition checking}.
The verifier does not re-solve the problem; instead, it checks whether the proposed next action is coherent with the verified state, whether variables are defined, whether the chosen action type matches the actual gap, and whether the action is mathematically safe to execute.
This gives MATH a strong pre-execution guardrail against forcing computation when a strategic retrieval step is still needed.

For GPQA, verification is split into two complementary levels.
The move verifier checks whether a proposed \texttt{<move>} is an actually executable next-step transition rather than a vague plan, requiring concrete checks and intermediate results.
The self-refine verifier then evaluates whether the accumulated reasoning trace sufficiently supports the current answer attempt and, if not, either requests targeted revision or explicitly recommends a new memory retrieval step.
This two-stage design is well suited to scientific question answering, where many failures arise from insufficiently decisive intermediate discrimination rather than from blatant formal invalidity.

For BigCodeBench, verification is specialized into lightweight static code checking.
The verifier checks whether the generated code respects the required interface, satisfies explicit constraints, and avoids obvious logical or syntactic failures, but it does not execute the code.
This reflects the role of verification in coding tasks as a pre-execution structural filter that catches mismatches in signature, return behavior, imports, or edge-case handling before expensive downstream evaluation.

\begin{tcolorbox}[
    breakable,
    colback=white!98!black,
    colframe=black!70!white,
    boxsep=4pt,
    top=2pt,
    title={\textbf{\large Function IX: Execution Specialist}},
    coltitle=black,
    colbacktitle=gray!20,
    bottom=2pt
]

\textbf{Execution Specialist Prompt Template}
\begin{lstlisting}[style=plainoutput]
You are the execution specialist for {domain} tasks.

[Input]
Approved request / implementation plan:
{request_or_plan}

[Task]
Execute the requested substep faithfully and produce the concrete artifact needed
by the planner.

Requirements:
1. Follow the approved scope only.
2. Do not re-plan the task at a higher level.
3. Return a domain-appropriate executable artifact or result.

[Output Format]
<analysis>
[Optional pre-flight check / scope check]
</analysis>

<result_or_artifact>
[Concrete calculation result, derivation result, or executable code]
</result_or_artifact>
\end{lstlisting}

\end{tcolorbox}

This function is present most explicitly in MATH and BigCodeBench, while GPQA relies more heavily on the planner itself plus optional calculation support.

For MATH, the execution specialist is specialized into a budget-constrained computational engine.
Before execution, it performs an atomic pre-flight analysis that parses the payload, selects a computation strategy, and checks hard limits such as symbolic complexity or iteration budgets.
Only then does it carry out the requested numeric or symbolic subtask.
This design ensures that calculator calls remain narrow, executable, and safe within competition-math settings.

For GPQA, execution is much lighter-weight at the prompt level.
Most local scientific reasoning steps are carried out directly through the planner's \texttt{<move>} action, while numeric or symbolic computation is delegated only when necessary.
As a result, GPQA places less emphasis on a dedicated execution-specialist prompt and more emphasis on deciding whether the next scientific check should be handled as retrieval, local reasoning, or computation.

For BigCodeBench, the execution specialist is specialized into a coding expert.
Rather than exploring alternatives, this agent receives the problem specification, interface constraints, and the planner's implementation blueprint, and converts them directly into executable Python code.
The prompt therefore emphasizes faithful realization of the approved plan, strict adherence to the target function signature, and explicit handling of the identified edge cases.

Overall, the three benchmarks share the same utilization pipeline: problem framing, online next-move planning, retrieval triggering, memory-grounded step synthesis, verification, and domain-specific execution.
The main differences lie in what constitutes a valid next step, how retrieval is formulated, and what kind of artifact the system must ultimately produce.
MATH emphasizes verified state transitions and strategic-vs-computational gap control, GPQA emphasizes discriminative next-step reasoning and trace-level self-refinement, and BigCodeBench emphasizes implementation planning, interface fidelity, and code-level execution support.
